# Supplementary material for: LiveView: Dynamic Target-Centered MPI for View Synthesis
Source: arXiv:2107.05113 source file (2021-07-11)
Supplement: Supplementary file 1 [file supplementary_10_view.tex]

\begin{figure*}
     \centering
     \begin{subfigure}
         \centering
         \includegraphics[width=\textwidth]{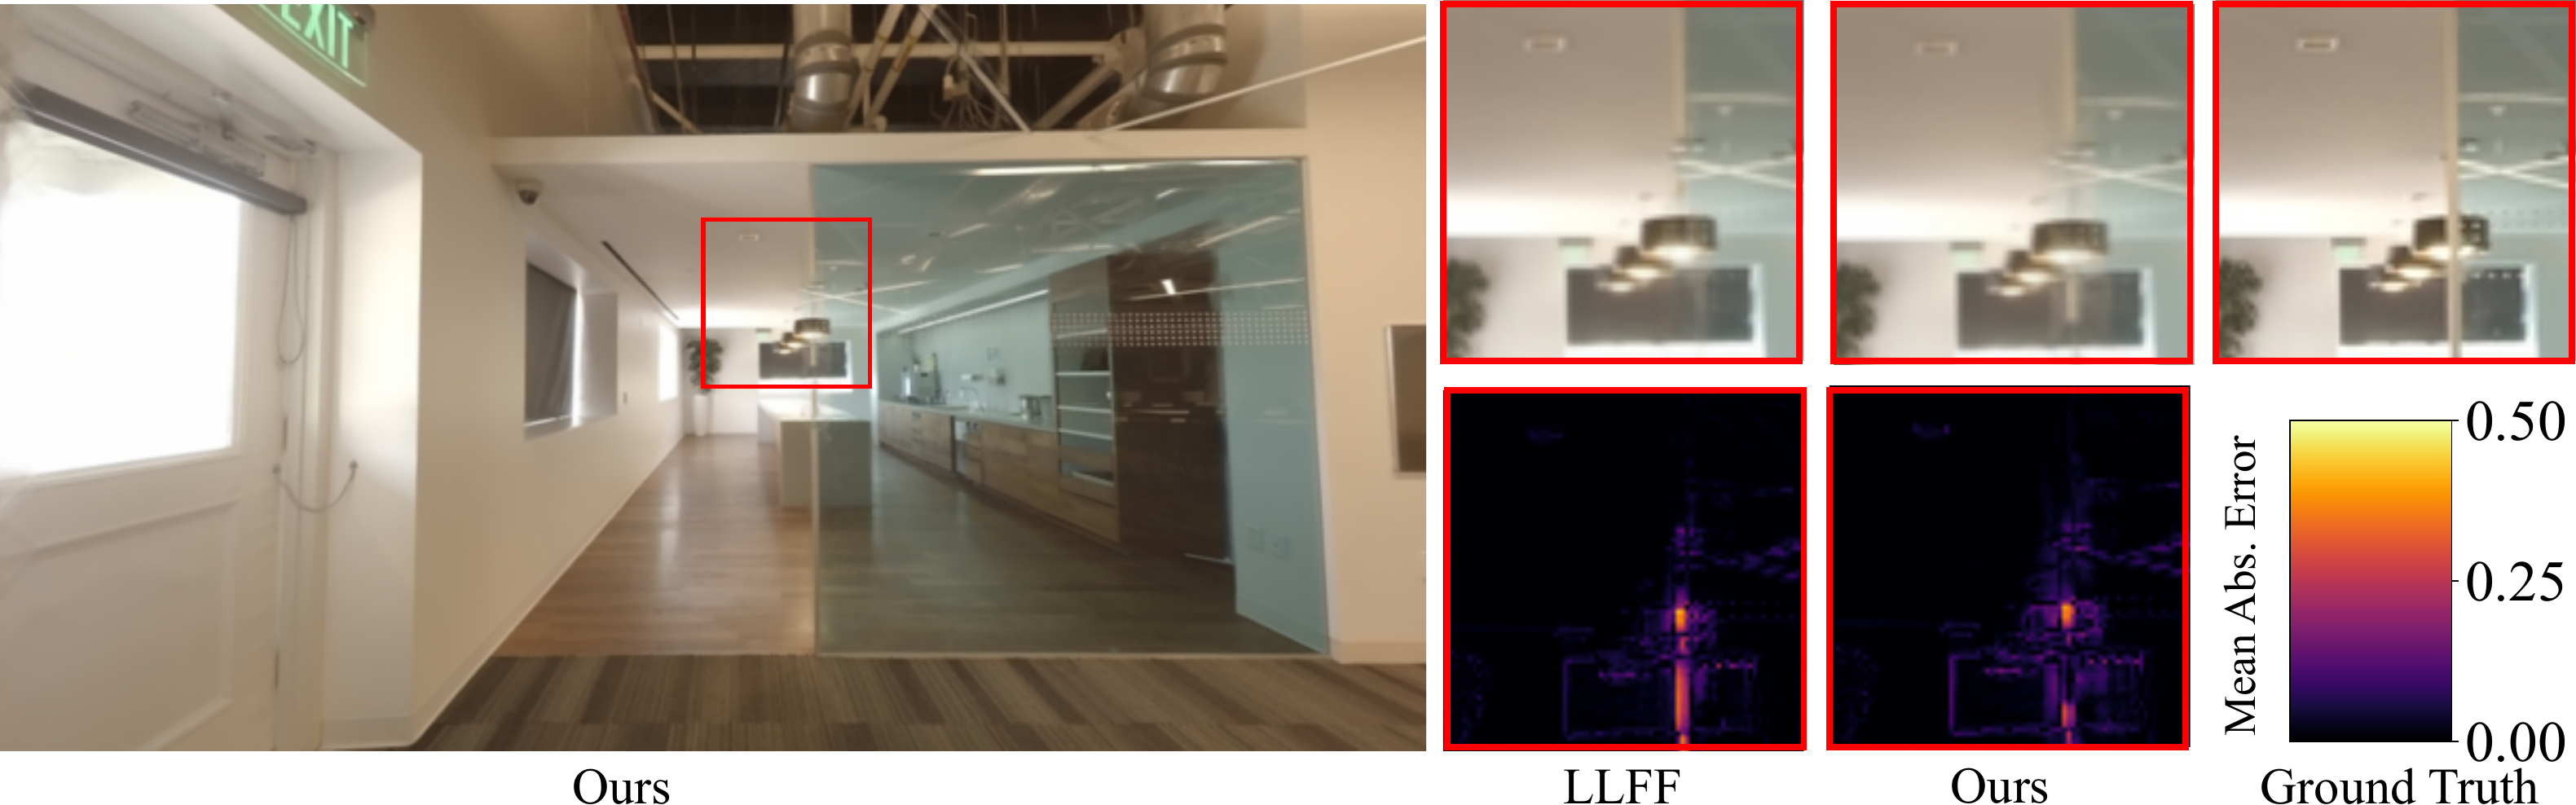}
     \end{subfigure}
     \hfill
     \begin{subfigure}
         \centering
         \includegraphics[width=\textwidth]{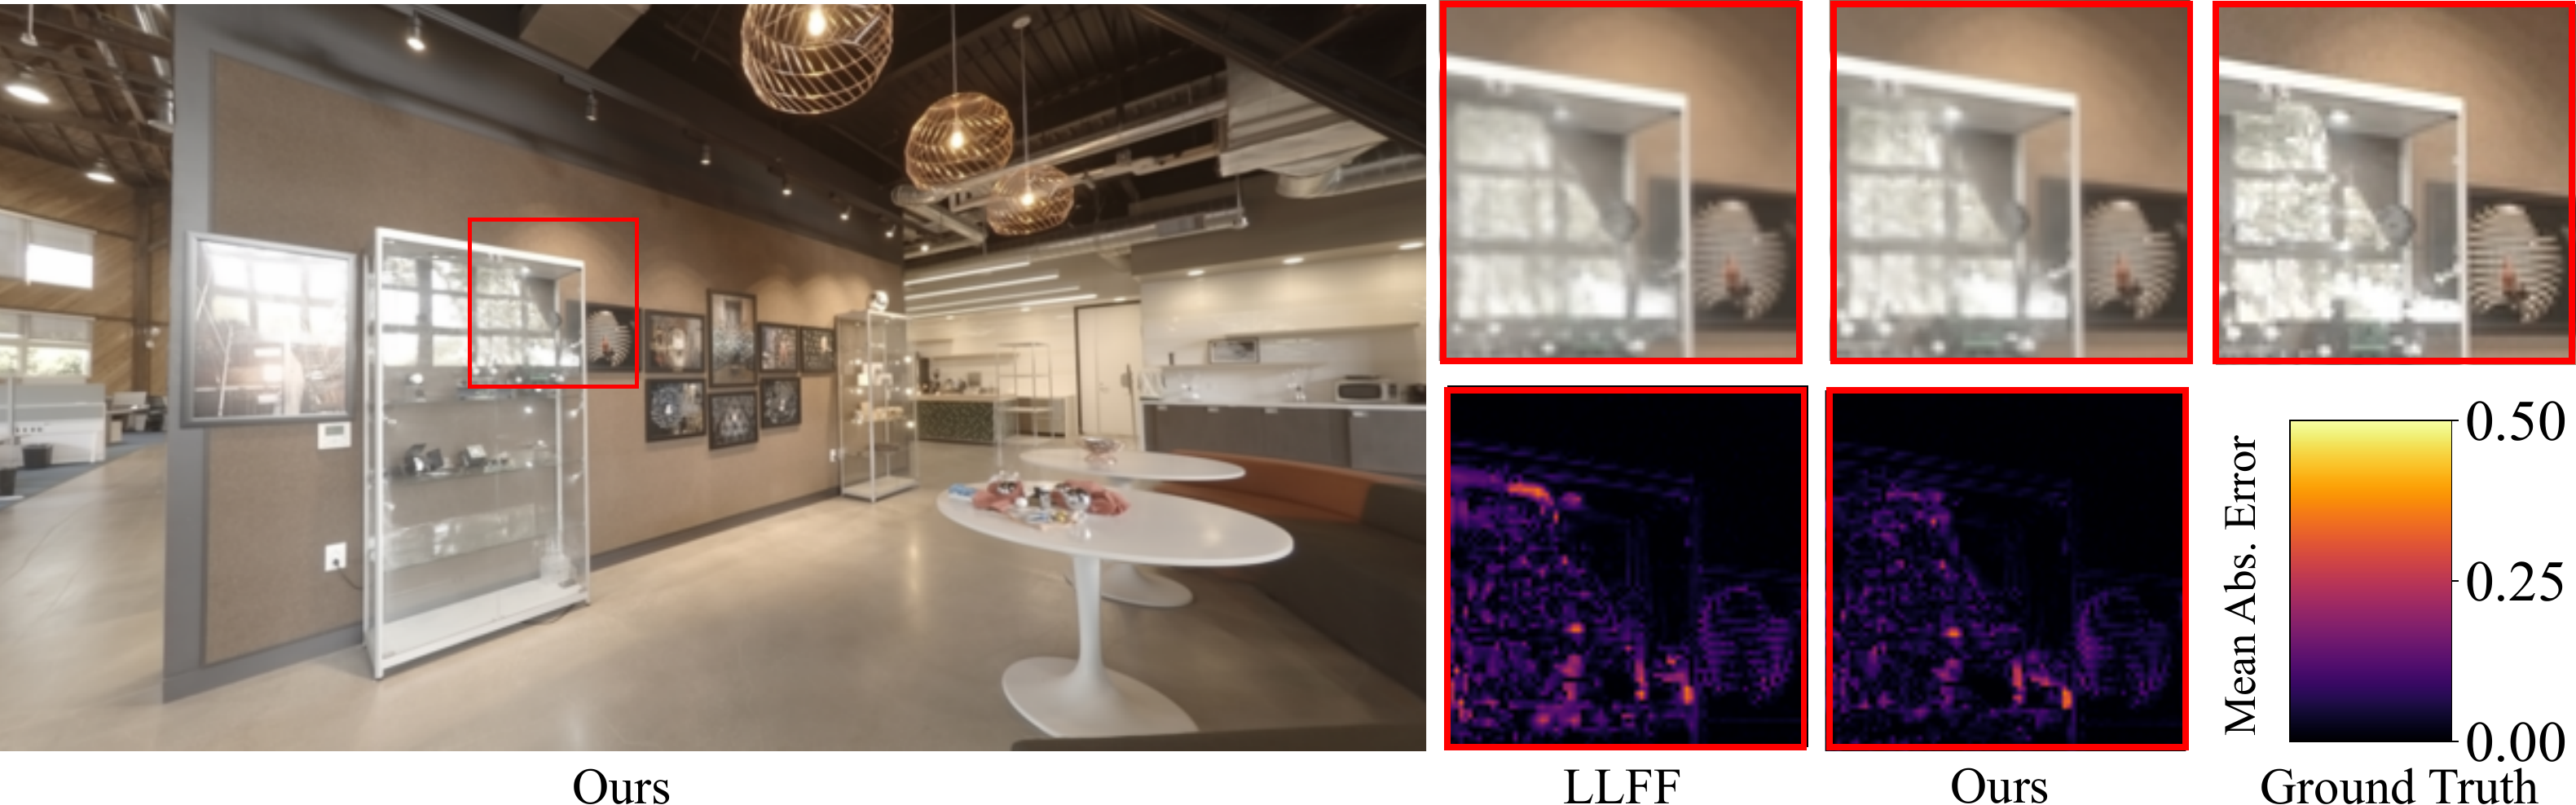}
     \end{subfigure}
     \hfill
     \begin{subfigure}
         \centering
         \includegraphics[width=\textwidth]{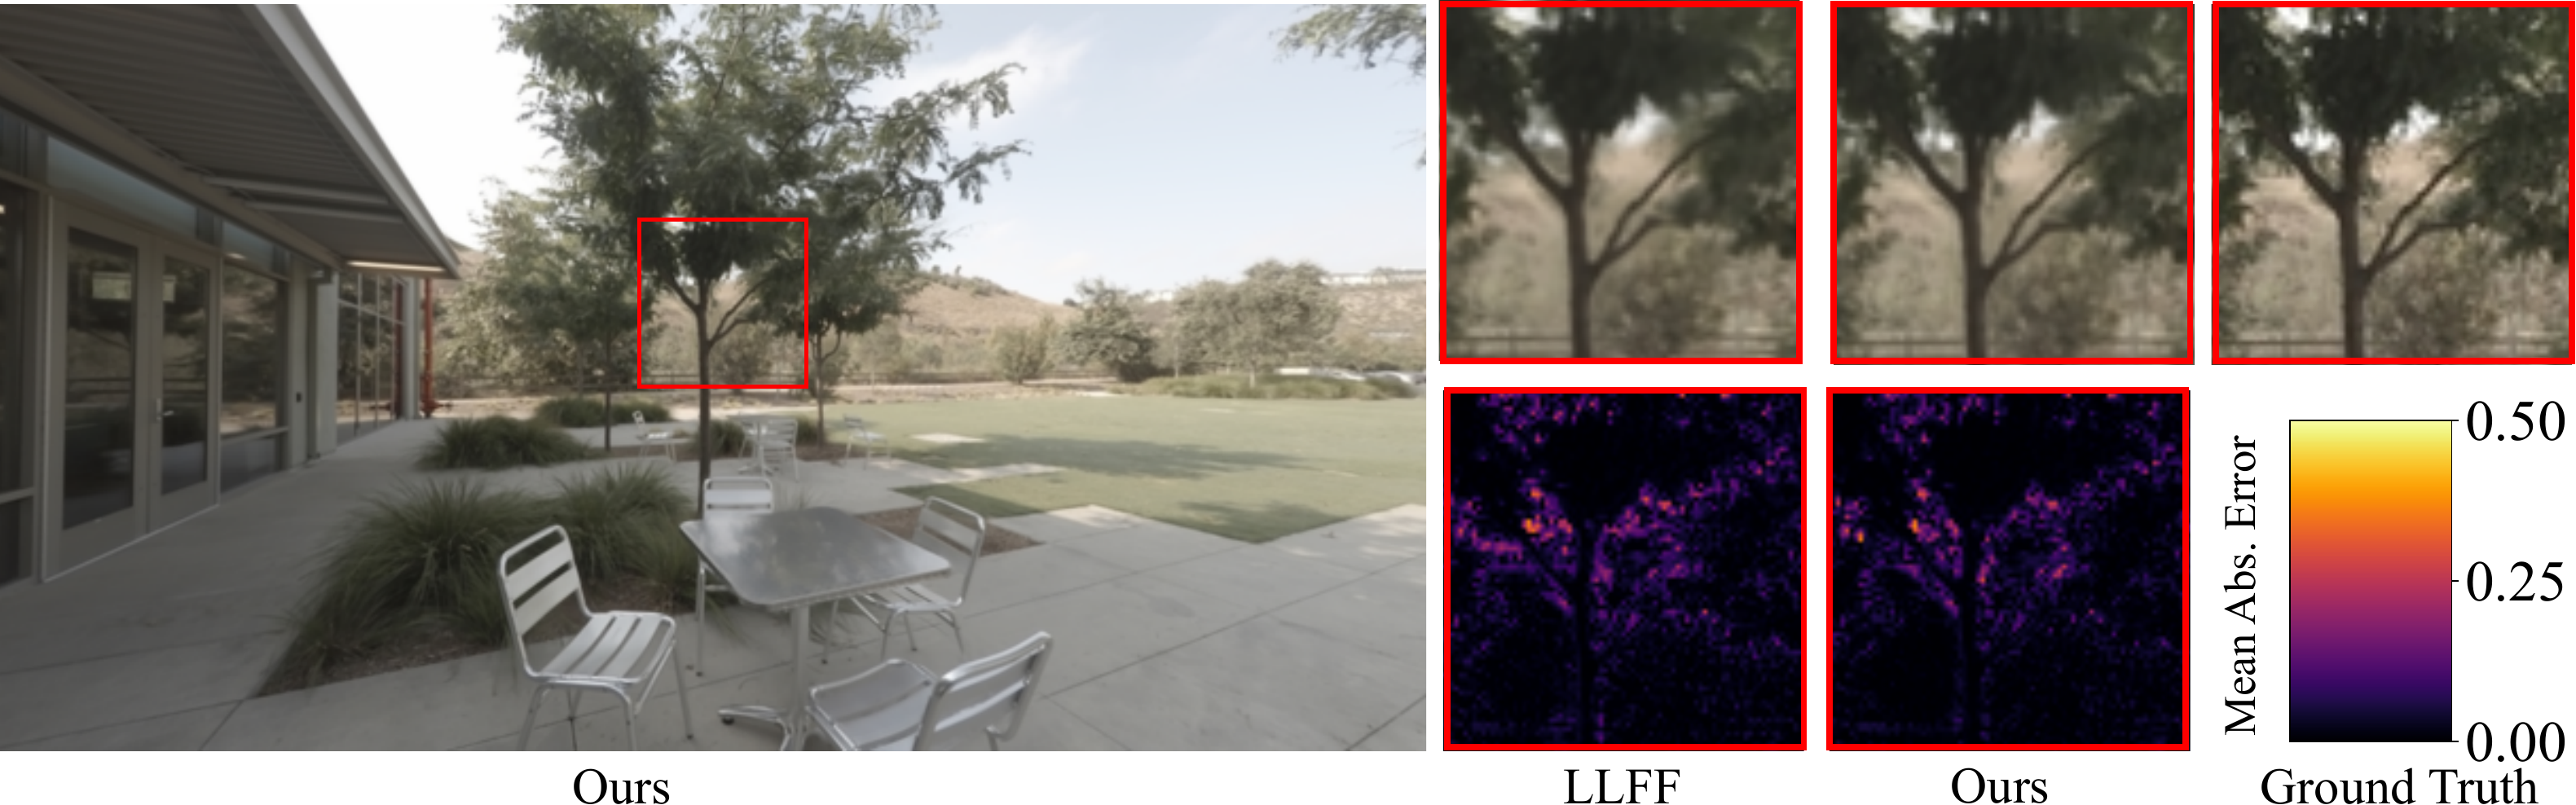}
     \end{subfigure}
     \begin{subfigure}
         \centering
         \includegraphics[width=\textwidth]{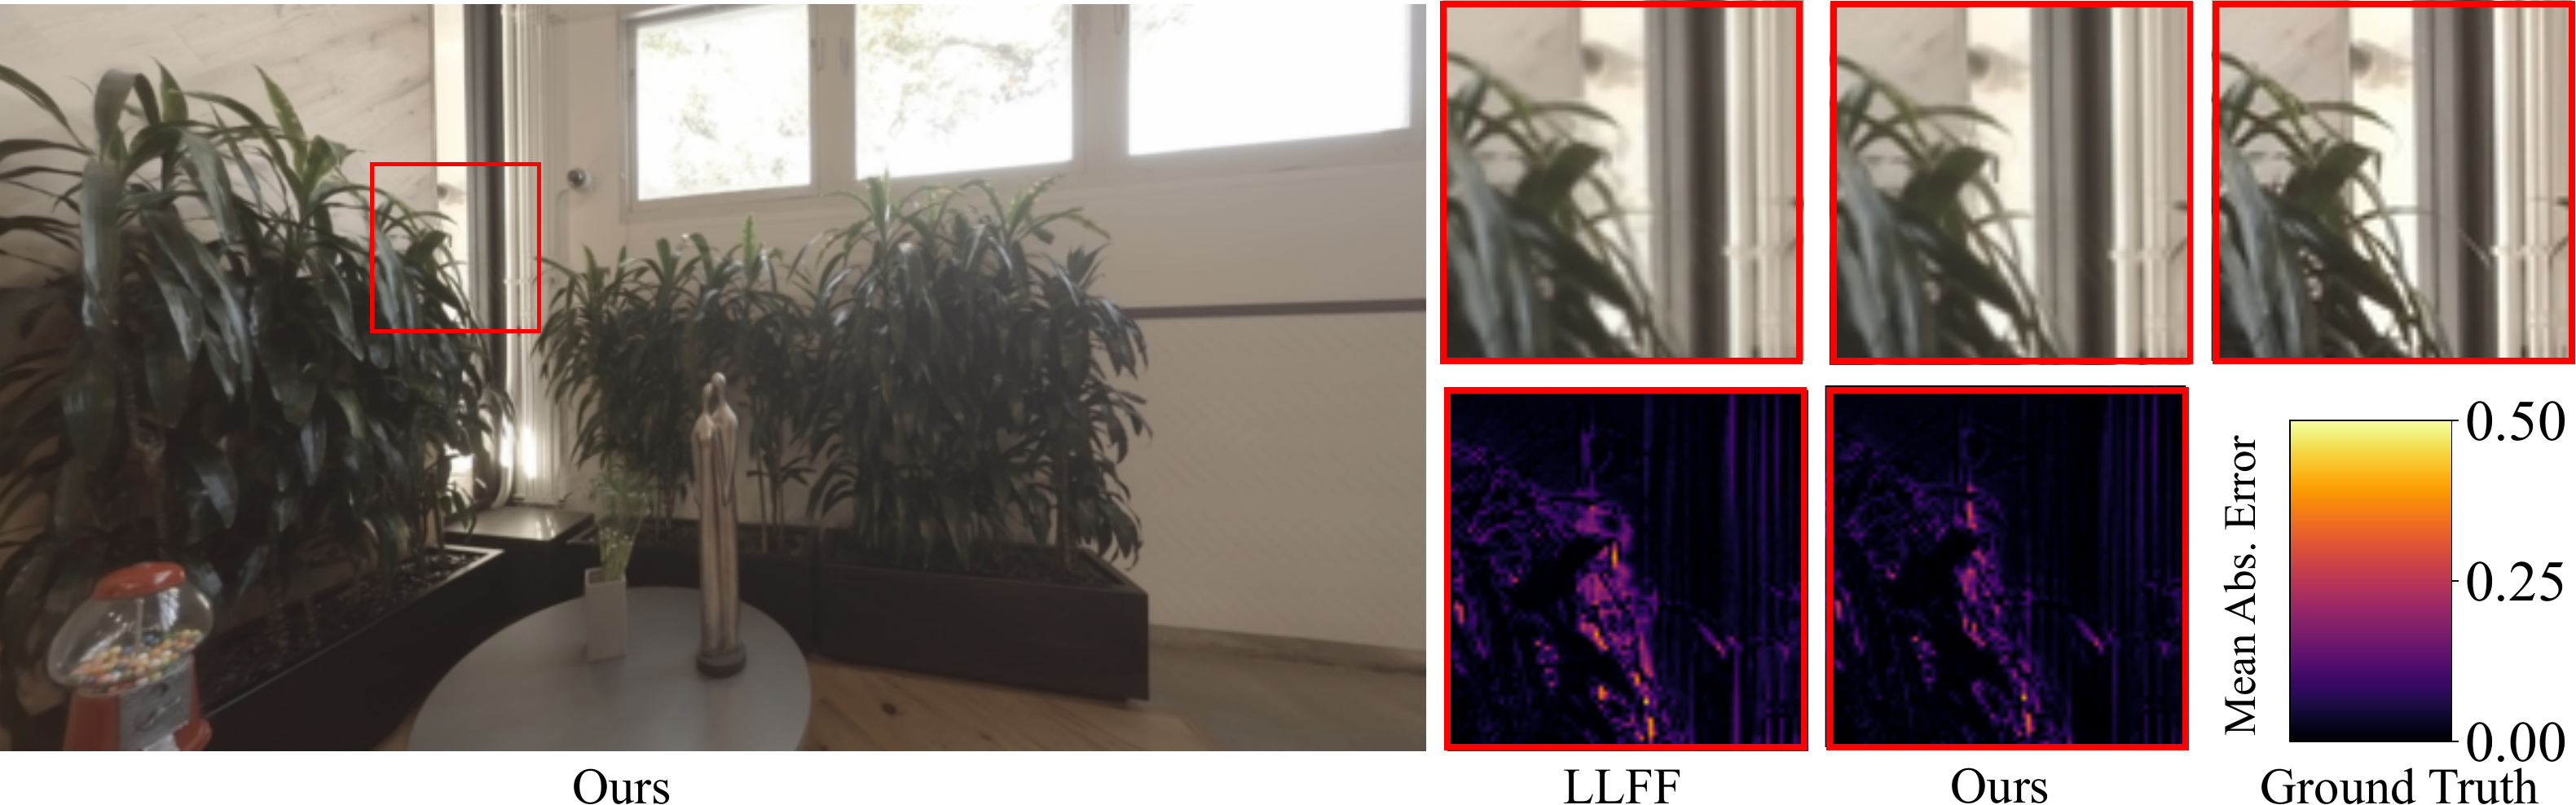}
     \end{subfigure}
     \caption{Comparison of 10 input configuration using our dynamic target-centered view synthesis and static input-centered LLFF~\cite{mildenhall2019local}. Inset shows a zoom in with the absolute difference map below it.}
    \label{fig:10_view}
\end{figure*}
