# Supplementary material for: LiveView: Dynamic Target-Centered MPI for View Synthesis
Source: arXiv:2107.05113 source file (2021-07-11)
Supplement: Supplementary file 2 [file supplementary_5_view.tex]

\begin{figure*}
     \centering
     \begin{subfigure}
         \centering
         \includegraphics[width=\textwidth]{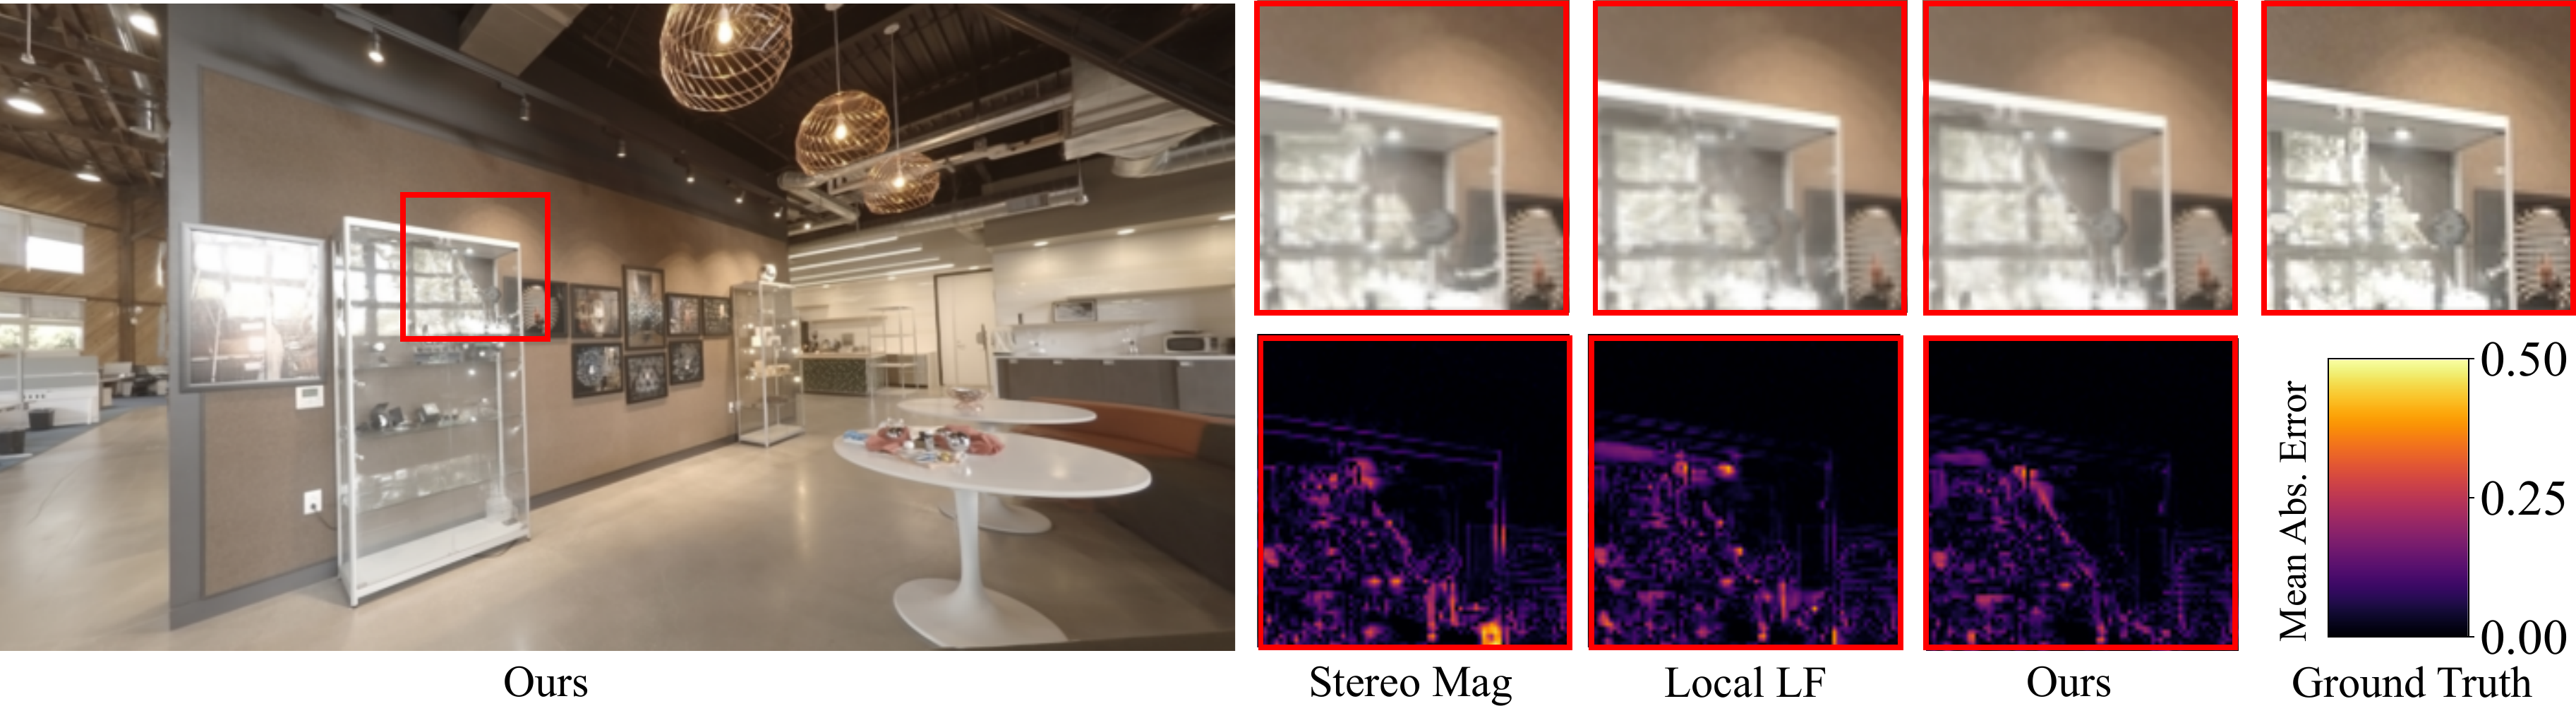}
     \end{subfigure}
     \begin{subfigure}
         \centering
         \includegraphics[width=\textwidth]{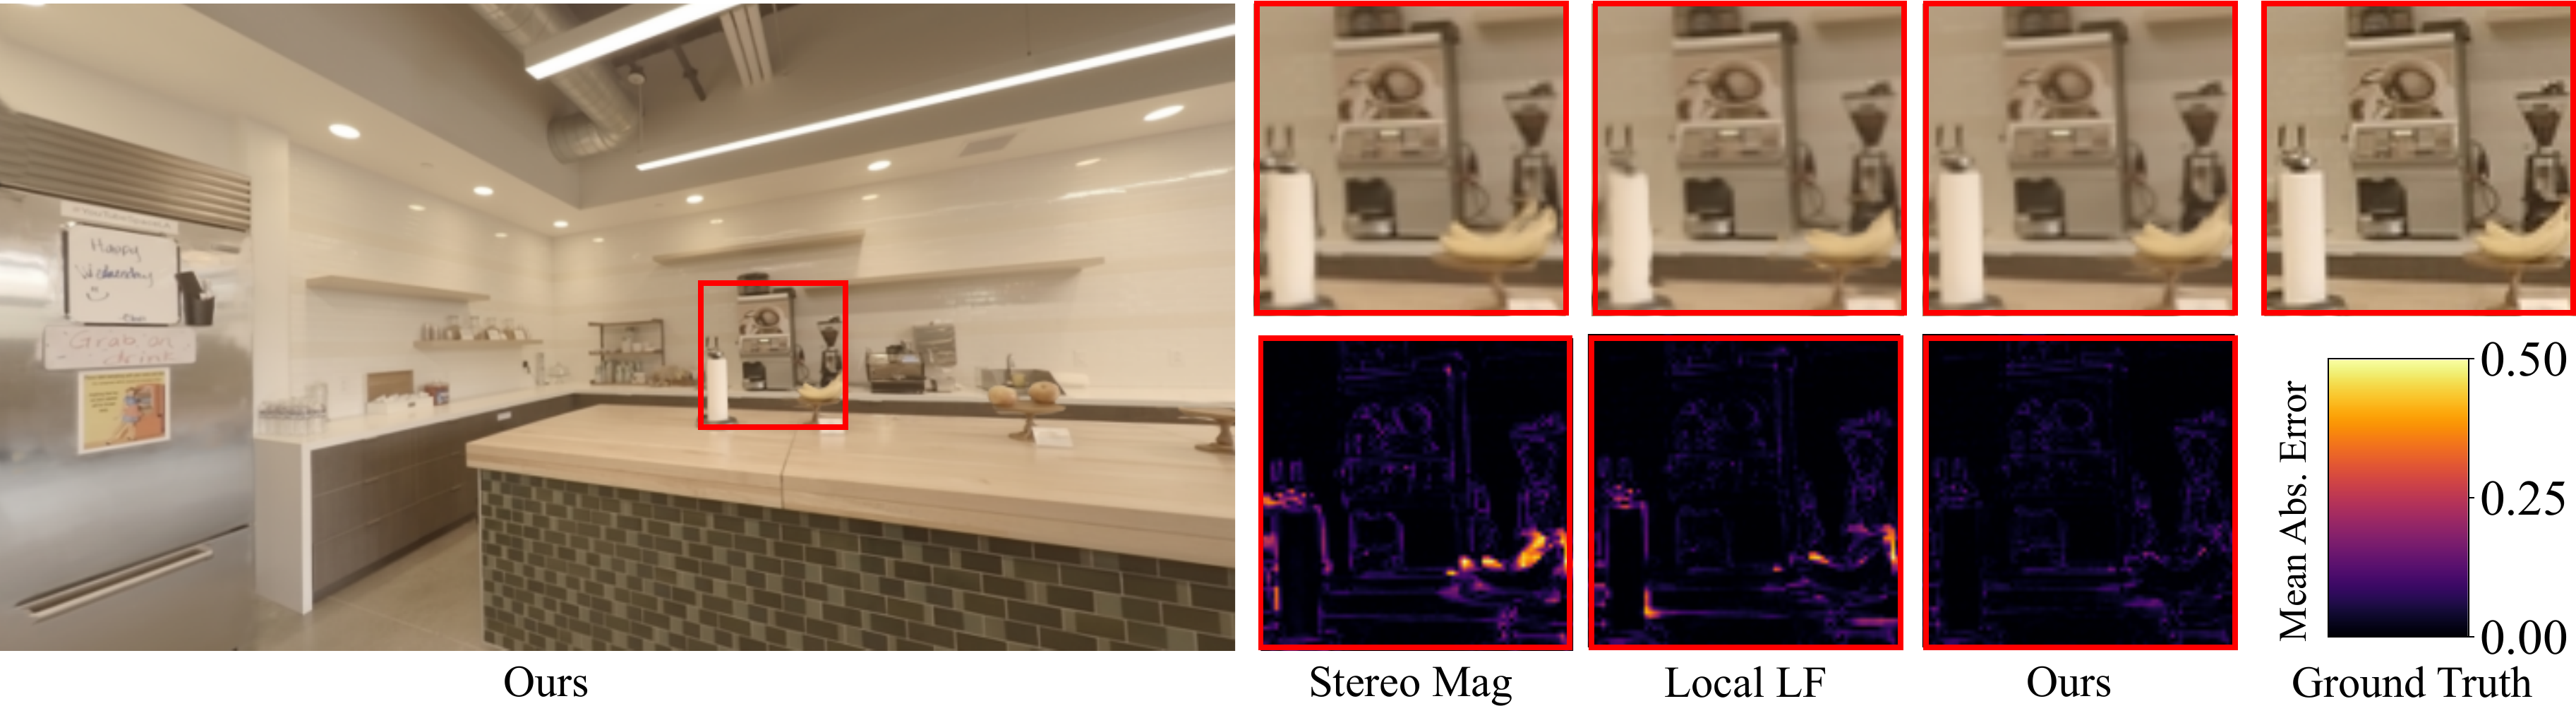}
     \end{subfigure}
     \begin{subfigure}
         \centering
         \includegraphics[width=\textwidth]{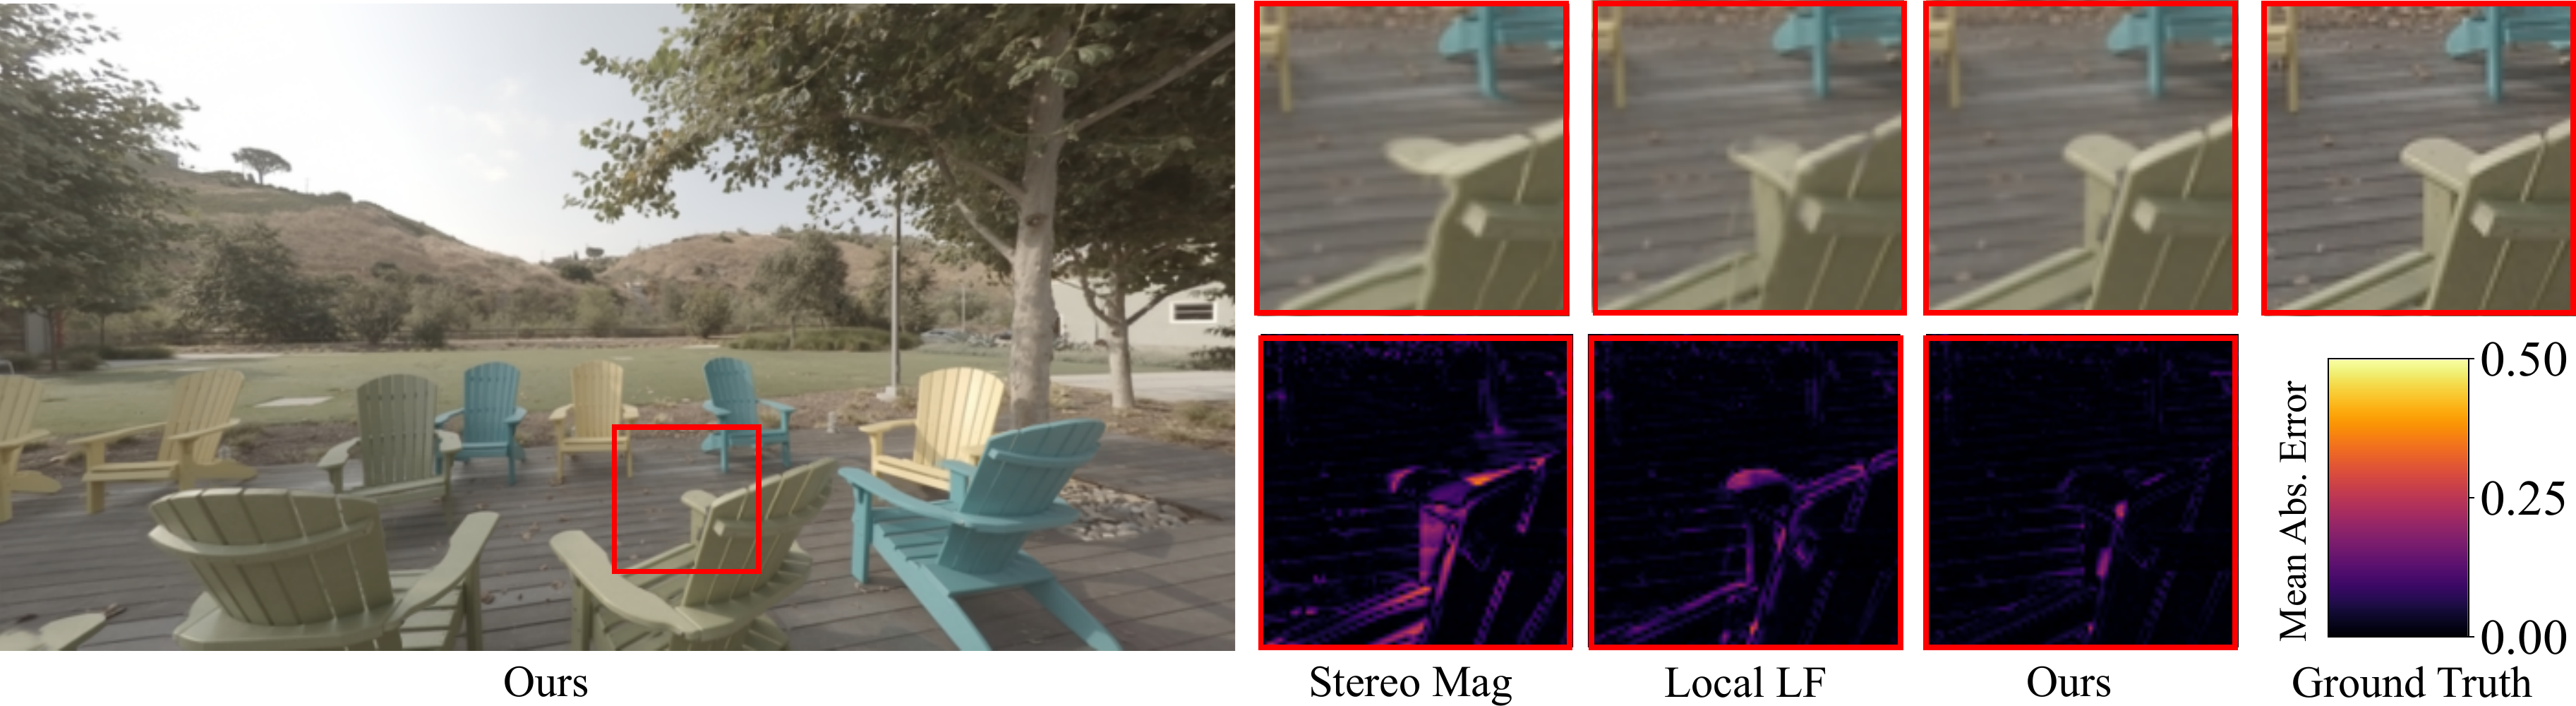}
     \end{subfigure}
     \begin{subfigure}
         \centering
         \includegraphics[width=\textwidth]{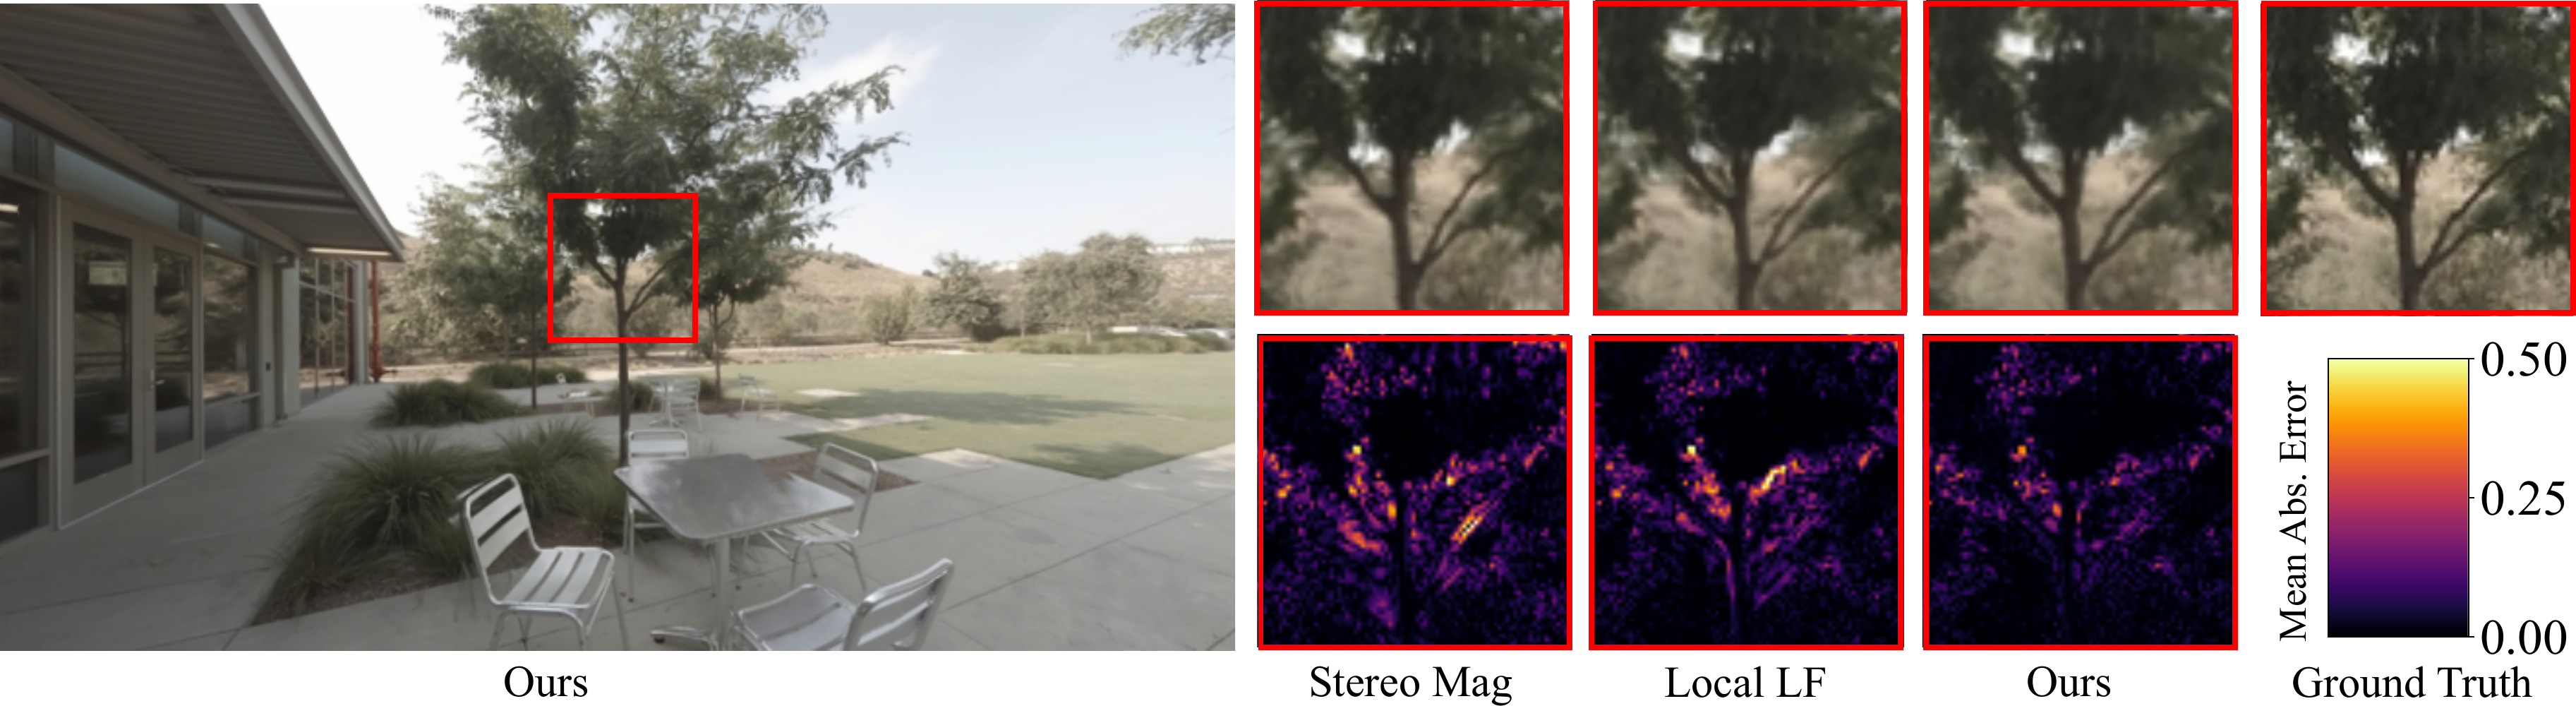}
     \end{subfigure}
        \caption{Comparison of our dynamic target-centered view synthesis and static input-centered view synthesis using both, Stereo Magnification ~\cite{zhou2018stereo} Local LF (base network for LLFF~\cite{mildenhall2019local}). Results are shown for 5 view input configuration. Inset shows a zoom in with the absolute difference map below it.}
        \label{fig:5_view}
\end{figure*}
